# Supplementary material for: Are Large Language Models Table-based Fact-Checkers?
Source: arXiv:2402.02549 source file (2024-11-13)
Supplement: Supplementary file 1 [file IEEEAppendix.tex]

\appendix

\section{Artifact Description Appendix: [Paper Title]}

%%%%%%%%%%%%%%%%%%%%%%%%%%%%%%%%%%%%%%%%%%%%%%%%%%%%%%%%%%%%%%%%%%%%%
\subsection{Abstract}

{\em If a paper has no artifact and submits this appendix, the authors only need to complete this abstract subsection and mention that the paper has no artifact.  This text is sufficient: \textbf{``This paper is not paired with an artifact.''}  Other subsections can be removed. In order to maintain consistency in naming conventions with the SC18 technical program, please consider the word "experiment" to be equivalent to "demonstration"}

%%%%%%%%%%%%%%%%%%%%%%%%%%%%%%%%%%%%%%%%%%%%%%%%%%%%%%%%%%%%%%%%%%%%%
\subsection{Description}

\subsubsection{Check-list (artifact meta information)}

{\em Fill in whatever is applicable with some informal keywords and remove the rest}

{\small
\begin{itemize}
  \item {\bf Algorithm: }
  \item {\bf Program: }
  \item {\bf Compilation: }
  \item {\bf Transformations: }
  \item {\bf Binary: }
  \item {\bf Data set: }
  \item {\bf Run-time environment: }
  \item {\bf Hardware: }
  \item {\bf Run-time state: }
  \item {\bf Execution: }
  \item {\bf Output: }
  \item {\bf Experiment workflow: }
  \item {\bf Experiment customization: }
  \item {\bf Publicly available?: }
  \item {\bf Wiring Diagrams: }
  \item {\bf Data Flow Descriptions: }
  
\end{itemize}
}
{\em Please pay special attention to obligatory descriptions below.}

\subsubsection{How software can be obtained }
{\em Obligatory if the paper is paired with an artifact.}

\subsubsection{Hardware dependencies}

\subsubsection{Software dependencies}
{\em Obligatory if the paper is paired with an artifact.}

\subsubsection{Datasets}

%%%%%%%%%%%%%%%%%%%%%%%%%%%%%%%%%%%%%%%%%%%%%%%%%%%%%%%%%%%%%%%%%%%%%
\subsection{Installation}

{\em Obligatory if the paper is paired with an artifact.}

%%%%%%%%%%%%%%%%%%%%%%%%%%%%%%%%%%%%%%%%%%%%%%%%%%%%%%%%%%%%%%%%%%%%%
\subsection{Experiment workflow}

{\em Obligatory if the paper is paired with an artifact.}

%%%%%%%%%%%%%%%%%%%%%%%%%%%%%%%%%%%%%%%%%%%%%%%%%%%%%%%%%%%%%%%%%%%%%
\subsection{Evaluation and expected result}

%%%%%%%%%%%%%%%%%%%%%%%%%%%%%%%%%%%%%%%%%%%%%%%%%%%%%%%%%%%%%%%%%%%%%
\subsection{Experiment customization}

%%%%%%%%%%%%%%%%%%%%%%%%%%%%%%%%%%%%%%%%%%%%%%%%%%%%%%%%%%%%%%%%%%%%%
\subsection{Notes}
